# Supplementary material for: Benchmarking World-Model Learning with Environment-Level Queries
Source: arXiv:2510.19788 source file (2026-05-07)
Supplement: Supplementary file 1 [file main-appendix-aux.tex]

\begin{filecontents}
{main-appendix.aux}
\relax 
\providecommand\hyper@newdestlabel[2]{}
\providecommand\HyField@AuxAddToFields[1]{}
\providecommand\HyField@AuxAddToCoFields[2]{}
\providecommand\BKM@entry[2]{}
\BKM@entry{id=1,dest={617070656E6469782E32},srcline={1}}{5C3337365C3337375C303030545C303030685C303030655C3030305C3034305C303030415C303030755C303030745C303030755C3030306D5C3030306E5C3030305C3034305C3030304C5C303030615C3030306E5C303030675C303030755C303030615C303030675C30303065}
\citation{autumnsynth}
\providecommand\csxdef[2]{}
\@writefile{toc}{\providecommand\autonum@processReference[2]{}}
\@writefile{lof}{\providecommand\autonum@processReference[2]{}}
\@writefile{toc}{\contentsline {section}{\numberline {A}The Autumn Language}{1}{appendix.2}\protected@file@percent }
\newlabel{sec:autumn}{{A}{1}{}{appendix.2}{}}
\newlabel{sec:autumn@cref}{{[appendix][1][]A}{[1][1][]1}{}{}{}}
\@writefile{toc}{\contentsline {paragraph}{Example Autumn Environment.}{1}{Item.5}\protected@file@percent }
\csxdef {autonum@lst:autumn_light_bar_exampleReferenced}{}
\csxdef {autonum@fig:treasure_environmentReferenced}{}
\savepointas{setupstart}{pgfid1}{0pt}{0pt}
\savepicturepage{pgfid1}{1}
\pgfsyspdfmark {pgfid1}{3646961}{20303547}
\savepointas{setupend}{pgfid2}{0pt}{0pt}
\savepicturepage{pgfid2}{1}
\pgfsyspdfmark {pgfid2}{12612263}{20303547}
\savepointas{objectstart}{pgfid3}{0pt}{0pt}
\savepicturepage{pgfid3}{1}
\pgfsyspdfmark {pgfid3}{3646961}{19386043}
\savepointas{objectend}{pgfid4}{0pt}{0pt}
\savepicturepage{pgfid4}{1}
\pgfsyspdfmark {pgfid4}{19690133}{17551035}
\savepointas{oninstancestart}{pgfid5}{0pt}{0pt}
\savepicturepage{pgfid5}{1}
\pgfsyspdfmark {pgfid5}{3646961}{16633531}
\savepointas{oninstanceend}{pgfid6}{0pt}{0pt}
\savepicturepage{pgfid6}{1}
\pgfsyspdfmark {pgfid6}{23229068}{13422267}
\savepointas{onstart}{pgfid7}{0pt}{0pt}
\savepicturepage{pgfid7}{1}
\pgfsyspdfmark {pgfid7}{3646961}{12504763}
\savepointas{onend}{pgfid8}{0pt}{0pt}
\savepicturepage{pgfid8}{1}
\pgfsyspdfmark {pgfid8}{20633849}{9752251}
\savepicturepage{pgfid9}{1}
\pgfsyspdfmark {pgfid9}{3646961}{8434976}
\@writefile{lol}{\contentsline {listing}{\numberline {A.1}{\ignorespaces A treasure-hunting environment example in Autumn.}}{1}{listing.caption.6}\protected@file@percent }
\providecommand*\caption@xref[2]{\@setref\relax\@undefined{#1}}
\newlabel{lst:autumn_light_bar_example}{{A.1}{1}{A treasure-hunting environment example in Autumn.\onlyinarxiv { Interactive demo available at \href {\detokenize {https://autumn.basis.ai/build-mode?code=KHByb2dyYW0KICAgKD0gR1JJRF9TSVpFIDUpCiAgIChvYmplY3QgUHJveGltaXR5ICg6IGRpc3QgTnVtYmVyKQogICAgIChtYXAgKC0tPiAoaSkgKENlbGwgaSAwIChpZiAoPD0gaSBkaXN0KSB0aGVuICJibHVlIiBlbHNlICJibGFjayIpKSkKICAgICAgICAgIChyYW5nZSAwIEdSSURfU0laRSkpKQogICAob2JqZWN0IFRyZWFzdXJlICg6IHJldmVhbGVkIEJvb2wpIChDZWxsIDAgMCAoaWYgcmV2ZWFsZWQgdGhlbiAiZ29sZCIgZWxzZSAiYmxhY2siKSkpCiAgIChvYmplY3QgQWdlbnQgKENlbGwgMCAwICJncmV5IikpCgogICAoOiB0cmVhc3VyZXMgKExpc3QgVHJlYXN1cmUpKQogICAoPSB0cmVhc3VyZXMgKGluaXRuZXh0IChsZXQKICAgICg9IHBvczEgKHVuaWZvcm1DaG9pY2UgKHJlY3QgKFBvc2l0aW9uIDAgMSkgKFBvc2l0aW9uIEdSSURfU0laRSBHUklEX1NJWkUpKSkpCiAgICAoPSBwb3MyICh1bmlmb3JtQ2hvaWNlIChmaWx0ZXIgKC0tPiBwICghICgmICg9PSAoLi4gcCB4KSAoLi4gcG9zMSB4KSkgKD09ICguLiBwIHkpICguLiBwb3MxIHkpKSkpKSAocmVjdCAoUG9zaXRpb24gMCAxKSAoUG9zaXRpb24gR1JJRF9TSVpFIEdSSURfU0laRSkpKSkpCiAgICAoPSBwb3MzICh1bmlmb3JtQ2hvaWNlIChmaWx0ZXIgKC0tPiBwICghICgmIChpbiAoLi4gcCB4KSAobGlzdCAoLi4gcG9zMSB4KSAoLi4gcG9zMiB4KSkpIChpbiAoLi4gcCB5KSAobGlzdCAoLi4gcG9zMSB5KSAoLi4gcG9zMiB5KSkpKSkpIChyZWN0IChQb3NpdGlvbiAwIDEpIChQb3NpdGlvbiBHUklEX1NJWkUgR1JJRF9TSVpFKSkpKSkKICAgIChwcmludCBwb3MzKQogICAgKGxpc3QgKFRyZWFzdXJlIHRydWUgcG9zMSkgKFRyZWFzdXJlIHRydWUgcG9zMikgKFRyZWFzdXJlIGZhbHNlIHBvczMpKQogICApIChwcmV2IHRyZWFzdXJlcykpKQoKICAgKDogYWdlbnQgQWdlbnQpCiAgICg9IGFnZW50IChpbml0bmV4dCAoQWdlbnQgKFBvc2l0aW9uIDAgMSkpIChwcmV2IGFnZW50KSkpCgogICA7IGNhbGN1bGF0ZSB0aGUgZGlzdGFuY2UgdG8gdGhlIGNsb3Nlc3QgdHJlYXN1cmUKICAgKD0gdGRpc3QgKGZuICh0cmVhc3VyZXMpCiAgICAoc3FkaXN0ICguLiBhZ2VudCBvcmlnaW4pICguLiAoY2xvc2VzdCBhZ2VudCB0cmVhc3VyZXMpIG9yaWdpbikpCiAgICkpCgogICAoOiBwcm94aW1pdHkgUHJveGltaXR5KQogICAoPSBwcm94aW1pdHkgKGluaXRuZXh0IChQcm94aW1pdHkgMiAoUG9zaXRpb24gMCAwKSkKICAgICAgKHVwZGF0ZU9iaiBwcm94aW1pdHkgImRpc3QiICgrICh0ZGlzdCB0cmVhc3VyZXMpICgtICh1bmlmb3JtQ2hvaWNlIChyYW5nZSAwIDMpKSAxKSkpKSkKCiAgIChvbiB1cCAoPSBhZ2VudCAobW92ZVVwIGFnZW50KSkpCiAgIChvbiBkb3duICg9IGFnZW50IChtb3ZlRG93biBhZ2VudCkpKQogICAob24gbGVmdCAoPSBhZ2VudCAobW92ZUxlZnQgYWdlbnQpKSkKICAgKG9uIHJpZ2h0ICg9IGFnZW50IChtb3ZlUmlnaHQgYWdlbnQpKSkKICAgKG9uIChjbGlja2VkIHRyZWFzdXJlcykgKD0gdHJlYXN1cmVzICh1cGRhdGVPYmogdHJlYXN1cmVzICgtLT4gb2JqICh1cGRhdGVPYmogb2JqICJyZXZlYWxlZCIgdHJ1ZSkpICgtLT4gb2JqIChjbGlja2VkIG9iaikpKSkpCiAgKQo=}}{\texttt {autumn.basis.ai}.}}}{listing.caption.6}{}}
\newlabel{lst:autumn_light_bar_example@cref}{{[listing][1][1]A.1}{[1][1][]1}{}{}{}}
\BKM@entry{id=2,dest={617070656E6469782E3333},srcline={121}}{5C3337365C3337375C303030415C303030755C303030745C303030755C3030306D5C3030306E5C303030425C303030655C3030306E5C303030635C303030685C3030305C3034305C303030455C3030306E5C303030765C303030695C303030725C3030306F5C3030306E5C3030306D5C303030655C3030306E5C303030745C3030305C3034305C303030445C303030655C303030745C303030615C303030695C3030306C5C30303073}
\@writefile{lof}{\contentsline {figure}{\numberline {A.1}{\ignorespaces Renderings of a partial trajectory of the Autumn environment example from \autonum@processReference {autonum@referenceCrefOld}{forcsvlist}{lst:autumn_light_bar_example}, following the sequence of actions down, down, down and click(1, 4).}}{2}{figure.caption.32}\protected@file@percent }
\csxdef {autonum@lst:autumn_light_bar_exampleReferenced}{}
\newlabel{fig:treasure_environment}{{A.1}{2}{Renderings of a partial trajectory of the Autumn environment example from \Cref {lst:autumn_light_bar_example}, following the sequence of actions down, down, down and click(1, 4)}{figure.caption.32}{}}
\newlabel{fig:treasure_environment@cref}{{[figure][1][1]A.1}{[1][1][]2}{}{}{}}
\@writefile{toc}{\contentsline {section}{\numberline {B}AutumnBench Environment Details}{2}{appendix.33}\protected@file@percent }
\newlabel{sec:env_details}{{B}{2}{}{appendix.33}{}}
\newlabel{sec:env_details@cref}{{[appendix][2][]B}{[1][2][]2}{}{}{}}
\csxdef {autonum@tab:env_categoriesReferenced}{}
\csxdef {autonum@tab:program_statsReferenced}{}
\@writefile{lot}{\contentsline {table}{\numberline {B.1}{\ignorespaces Category tags for each AutumnBench environment. Labels are non-exclusive.}}{3}{table.caption.34}\protected@file@percent }
\newlabel{tab:env_categories}{{B.1}{3}{Category tags for each AutumnBench environment. Labels are non-exclusive}{table.caption.34}{}}
\newlabel{tab:env_categories@cref}{{[table][1][2]B.1}{[1][2][]3}{}{}{}}
\@writefile{lot}{\contentsline {table}{\numberline {B.2}{\ignorespaces Program statistics for all AutumnBench environments. Columns: number of object types (\#Obj), number of latent variables (\#Lat., i.e.\ Autumn program fields not rendered on the grid), program length in lines of code (Len.), number of event handlers (\#On), number of colors (\#Col.), and grid size. \textbf  {Left:} deterministic environments. \textbf  {Right:} stochastic environments.}}{3}{table.caption.35}\protected@file@percent }
\newlabel{tab:program_stats}{{B.2}{3}{Program statistics for all AutumnBench environments. Columns: number of object types (\#Obj), number of latent variables (\#Lat., i.e.\ Autumn program fields not rendered on the grid), program length in lines of code (Len.), number of event handlers (\#On), number of colors (\#Col.), and grid size. \textbf {Left:} deterministic environments. \textbf {Right:} stochastic environments}{table.caption.35}{}}
\newlabel{tab:program_stats@cref}{{[table][2][2]B.2}{[1][2][]3}{}{}{}}
\BKM@entry{id=3,dest={617070656E6469782E3336},srcline={252}}{5C3337365C3337375C303030415C303030755C303030745C303030755C3030306D5C3030306E5C303030425C303030655C3030306E5C303030635C303030685C3030305C3034305C303030435C303030685C303030615C3030306C5C3030306C5C303030655C3030306E5C303030675C303030655C3030305C3034305C303030465C3030306F5C303030725C3030306D5C303030755C3030306C5C303030615C303030745C303030695C3030306F5C3030306E}
\BKM@entry{id=4,dest={73756273656374696F6E2E3337},srcline={257}}{5C3337365C3337375C3030304D5C303030615C303030735C3030306B5C303030655C303030645C3030305C3034305C303030465C303030725C303030615C3030306D5C303030655C3030305C3034305C303030505C303030725C303030655C303030645C303030695C303030635C303030745C303030695C3030306F5C3030306E}
\BKM@entry{id=5,dest={73756273656374696F6E2E3338},srcline={268}}{5C3337365C3337375C303030435C303030685C303030615C3030306E5C303030675C303030655C3030305C3034305C303030445C303030655C303030745C303030655C303030635C303030745C303030695C3030306F5C3030306E}
\BKM@entry{id=6,dest={73756273656374696F6E2E3431},srcline={290}}{5C3337365C3337375C303030505C3030306C5C303030615C3030306E5C3030306E5C303030695C3030306E5C30303067}
\BKM@entry{id=7,dest={617070656E6469782E3432},srcline={296}}{5C3337365C3337375C303030495C3030306D5C303030705C3030306C5C303030655C3030306D5C303030655C3030306E5C303030745C303030615C303030745C303030695C3030306F5C3030306E5C3030305C3034305C303030445C303030655C303030745C303030615C303030695C3030306C5C30303073}
\BKM@entry{id=8,dest={73756273656374696F6E2E3433},srcline={301}}{5C3337365C3337375C3030304E5C3030306F5C303030725C3030306D5C303030615C3030306C5C303030695C3030307A5C303030655C303030645C3030305C3034305C303030505C303030655C303030725C303030705C3030306C5C303030655C303030785C303030695C303030745C30303079}
\@writefile{toc}{\contentsline {section}{\numberline {C}AutumnBench Challenge Formulation}{4}{appendix.36}\protected@file@percent }
\newlabel{sec:challenge-formulation}{{C}{4}{}{appendix.36}{}}
\newlabel{sec:challenge-formulation@cref}{{[appendix][3][]C}{[1][4][]4}{}{}{}}
\@writefile{toc}{\contentsline {subsection}{\numberline {C.1}Masked Frame Prediction}{4}{subsection.37}\protected@file@percent }
\@writefile{toc}{\contentsline {subsection}{\numberline {C.2}Change Detection}{4}{subsection.38}\protected@file@percent }
\@writefile{toc}{\contentsline {subsection}{\numberline {C.3}Planning}{4}{subsection.41}\protected@file@percent }
\@writefile{toc}{\contentsline {section}{\numberline {D}Implementation Details}{4}{appendix.42}\protected@file@percent }
\newlabel{sec:impl_details}{{D}{4}{}{appendix.42}{}}
\newlabel{sec:impl_details@cref}{{[appendix][4][]D}{[1][4][]4}{}{}{}}
\BKM@entry{id=9,dest={73756273656374696F6E2E3436},srcline={324}}{5C3337365C3337375C303030545C303030615C303030735C3030306B5C3030305C3034305C303030495C3030306E5C303030745C303030655C303030725C303030665C303030615C303030635C303030655C3030305C3034305C303030495C3030306D5C303030705C3030306C5C303030655C3030306D5C303030655C3030306E5C303030745C303030615C303030745C303030695C3030306F5C3030306E}
\BKM@entry{id=10,dest={73756273756273656374696F6E2E3437},srcline={328}}{5C3337365C3337375C303030475C303030725C303030615C303030705C303030685C303030695C303030635C303030615C3030306C5C3030305C3034305C303030555C303030735C303030655C303030725C3030305C3034305C303030495C3030306E5C303030745C303030655C303030725C303030665C303030615C303030635C30303065}
\@writefile{toc}{\contentsline {subsection}{\numberline {D.1}Normalized Perplexity}{5}{subsection.43}\protected@file@percent }
\newlabel{def:norm_perplexity}{{D.1}{5}{Normalized Perplexity}{definition.1.D.1}{}}
\newlabel{def:norm_perplexity@cref}{{[definition][1][4]D.1}{[1][4][]5}{}{}{}}
\newlabel{def:auc}{{D.2}{5}{Area Under the Curve (AUC) of Normalized Perplexity}{definition.1.D.2}{}}
\newlabel{def:auc@cref}{{[definition][2][4]D.2}{[1][5][]5}{}{}{}}
\@writefile{toc}{\contentsline {subsection}{\numberline {D.2}Task Interface Implementation}{5}{subsection.46}\protected@file@percent }
\@writefile{toc}{\contentsline {subsubsection}{\numberline {D.2.1}Graphical User Interface}{5}{subsubsection.47}\protected@file@percent }
\newlabel{sec:task-gui}{{D.2.1}{5}{Final Normalized Perplexity}{subsubsection.47}{}}
\newlabel{sec:task-gui@cref}{{[subsubsection][1][4,2]D.2.1}{[1][5][]5}{}{}{}}
\@writefile{lof}{\contentsline {figure}{\numberline {D.1}{\ignorespaces Example of masked frame prediction task on the AutumnBench GUI showing the slider, action viewer, six choice options, and a \texttt  {Submit} button.}}{5}{figure.caption.48}\protected@file@percent }
\newlabel{fig:mfp-grid}{{D.1}{5}{Example of masked frame prediction task on the AutumnBench GUI showing the slider, action viewer, six choice options, and a \texttt {Submit} button}{figure.caption.48}{}}
\newlabel{fig:mfp-grid@cref}{{[figure][1][4]D.1}{[1][5][]5}{}{}{}}
\csxdef {autonum@fig:mfp-gridReferenced}{}
\@writefile{lof}{\contentsline {figure}{\numberline {D.2}{\ignorespaces Example of planning task on the AutumnBench GUI that shows a target region by masking out cells that are not in the target.}}{5}{figure.caption.49}\protected@file@percent }
\newlabel{fig:planning-grid}{{D.2}{5}{Example of planning task on the AutumnBench GUI that shows a target region by masking out cells that are not in the target}{figure.caption.49}{}}
\newlabel{fig:planning-grid@cref}{{[figure][2][4]D.2}{[1][5][]5}{}{}{}}
\csxdef {autonum@fig:planning-gridReferenced}{}
\@writefile{lof}{\contentsline {figure}{\numberline {D.3}{\ignorespaces Change detection on the AutumnBench GUI. (a) Initial change detection phase with \texttt  {Reset} and \texttt  {Found change} buttons. (b) Frame selection phase with the action viewer, slider, and \texttt  {Submit} button.}}{6}{figure.caption.50}\protected@file@percent }
\newlabel{fig:change-detection-grid}{{D.3}{6}{Change detection on the AutumnBench GUI. (a) Initial change detection phase with \texttt {Reset} and \texttt {Found change} buttons. (b) Frame selection phase with the action viewer, slider, and \texttt {Submit} button}{figure.caption.50}{}}
\newlabel{fig:change-detection-grid@cref}{{[figure][3][4]D.3}{[1][5][]6}{}{}{}}
\csxdef {autonum@fig:change-detection-gridReferenced}{}
\BKM@entry{id=11,dest={73756273756273656374696F6E2E3531},srcline={382}}{5C3337365C3337375C303030545C303030655C303030785C303030745C3030302D5C303030425C303030615C303030735C303030655C303030645C3030305C3034305C303030495C3030306E5C303030745C303030655C303030725C303030665C303030615C303030635C30303065}
\@writefile{toc}{\contentsline {subsubsection}{\numberline {D.2.2}Text-Based Interface}{7}{subsubsection.51}\protected@file@percent }
\newlabel{sec:text-interface}{{D.2.2}{7}{Final Normalized Perplexity}{subsubsection.51}{}}
\newlabel{sec:text-interface@cref}{{[subsubsection][2][4,2]D.2.2}{[1][7][]7}{}{}{}}
\csxdef {autonum@lst:sys-promptReferenced}{}
\csxdef {autonum@lst:mfp-promptReferenced}{}
\csxdef {autonum@lst:planning-promptReferenced}{}
\csxdef {autonum@lst:change-detection-promptReferenced}{}
\@writefile{lol}{\contentsline {listing}{\numberline {D.1}{\ignorespaces System prompt for all reasoning models}}{8}{listing.caption.52}\protected@file@percent }
\newlabel{lst:sys-prompt}{{D.1}{8}{System prompt for all reasoning models}{listing.caption.52}{}}
\newlabel{lst:sys-prompt@cref}{{[listing][1][4]D.1}{[1][7][]8}{}{}{}}
\@writefile{lol}{\contentsline {listing}{\numberline {D.2}{\ignorespaces Prompt for masked frame prediction task}}{8}{listing.caption.75}\protected@file@percent }
\newlabel{lst:mfp-prompt}{{D.2}{8}{Prompt for masked frame prediction task}{listing.caption.75}{}}
\newlabel{lst:mfp-prompt@cref}{{[listing][2][4]D.2}{[1][7][]8}{}{}{}}
\@writefile{lol}{\contentsline {listing}{\numberline {D.3}{\ignorespaces Prompts for change detection task}}{9}{listing.caption.89}\protected@file@percent }
\newlabel{lst:change-detection-prompt}{{D.3}{9}{Prompts for change detection task}{listing.caption.89}{}}
\newlabel{lst:change-detection-prompt@cref}{{[listing][3][4]D.3}{[1][7][]9}{}{}{}}
\@writefile{lol}{\contentsline {listing}{\numberline {D.4}{\ignorespaces Prompts for planning task}}{10}{listing.caption.108}\protected@file@percent }
\newlabel{lst:planning-prompt}{{D.4}{10}{Prompts for planning task}{listing.caption.108}{}}
\newlabel{lst:planning-prompt@cref}{{[listing][4][4]D.4}{[1][7][]10}{}{}{}}
\BKM@entry{id=12,dest={617070656E6469782E313232},srcline={482}}{5C3337365C3337375C303030545C303030685C303030655C3030306F5C303030725C303030655C303030745C303030695C303030635C303030615C3030306C5C3030305C3034305C303030465C303030725C303030615C3030306D5C303030655C303030775C3030306F5C303030725C3030306B5C3030305C3034305C303030615C3030306E5C303030645C3030305C3034305C303030525C303030655C303030665C303030655C303030725C303030655C3030306E5C303030635C303030655C3030305C3034305C303030425C303030615C303030735C303030655C3030306C5C303030695C3030306E5C303030655C30303073}
\BKM@entry{id=13,dest={73756273656374696F6E2E313233},srcline={487}}{5C3337365C3337375C303030545C303030685C303030655C3030306F5C303030725C303030655C303030745C303030695C303030635C303030615C3030306C5C3030305C3034305C303030465C303030725C303030615C3030306D5C303030655C303030775C3030306F5C303030725C3030306B5C3030305C3034305C303030665C3030306F5C303030725C3030305C3034305C3030304E5C303030655C303030785C303030745C3030302D5C303030535C303030745C303030615C303030745C303030655C3030305C3034305C303030505C303030725C303030655C303030645C303030695C303030635C303030745C303030695C3030306F5C3030306E5C3030305C3034305C3030304D5C3030306F5C303030645C303030655C3030306C5C30303073}
\BKM@entry{id=14,dest={73756273756273656374696F6E2E313234},srcline={492}}{5C3337365C3337375C3030304E5C303030655C303030785C303030745C3030302D5C303030535C303030745C303030615C303030745C303030655C3030305C3034305C303030505C303030725C303030655C303030645C303030695C303030635C303030745C303030695C3030306F5C3030306E5C3030305C3034305C3030304D5C3030306F5C303030645C303030655C3030306C}
\BKM@entry{id=15,dest={73756273656374696F6E2E313330},srcline={534}}{5C3337365C3337375C3030304E5C3030306F5C3030306E5C3030302D5C3030304C5C3030304C5C3030304D5C3030305C3034305C303030425C303030615C303030735C303030655C3030306C5C303030695C3030306E5C303030655C3030305C3034305C303030415C303030675C303030655C3030306E5C303030745C30303073}
\BKM@entry{id=16,dest={73756273756273656374696F6E2E313331},srcline={539}}{5C3337365C3337375C303030415C303030755C303030745C303030755C3030306D5C3030306E5C3030302D5C303030535C303030695C3030306D5C303030755C3030306C5C303030615C303030745C3030306F5C303030725C3030305C3034305C303030415C303030675C303030655C3030306E5C30303074}
\citation{dreamerv3}
\@writefile{toc}{\contentsline {section}{\numberline {E}Theoretical Framework and Reference Baselines}{11}{appendix.122}\protected@file@percent }
\csxdef {autonum@sec:theoretical-frameworkReferenced}{}
\csxdef {autonum@sec:autumn-simulator-agentReferenced}{}
\csxdef {autonum@sec:random-agent-resultsReferenced}{}
\@writefile{toc}{\contentsline {subsection}{\numberline {E.1}Theoretical Framework for Next-State Prediction Models}{11}{subsection.123}\protected@file@percent }
\newlabel{sec:theoretical-framework}{{E.1}{11}{Final Normalized Perplexity}{subsection.123}{}}
\newlabel{sec:theoretical-framework@cref}{{[appendix][1][5]E.1}{[1][11][]11}{}{}{}}
\csxdef {autonum@sec:autumn-simulator-agentReferenced}{}
\@writefile{toc}{\contentsline {subsubsection}{\numberline {E.1.1}Next-State Prediction Model}{11}{subsubsection.124}\protected@file@percent }
\newlabel{sec:next-state-prediction-model}{{E.1.1}{11}{Final Normalized Perplexity}{subsubsection.124}{}}
\newlabel{sec:next-state-prediction-model@cref}{{[subsubsection][1][5,1]E.1.1}{[1][11][]11}{}{}{}}
\@writefile{toc}{\contentsline {subsection}{\numberline {E.2}Non-LLM Baseline Agents}{11}{subsection.130}\protected@file@percent }
\newlabel{sec:baseline-agents}{{E.2}{11}{Final Normalized Perplexity}{subsection.130}{}}
\newlabel{sec:baseline-agents@cref}{{[appendix][2][5]E.2}{[1][11][]11}{}{}{}}
\csxdef {autonum@sec:autumn-simulator-agentReferenced}{}
\csxdef {autonum@sec:random-agent-resultsReferenced}{}
\BKM@entry{id=17,dest={73756273756273656374696F6E2E313332},srcline={556}}{5C3337365C3337375C303030525C303030615C3030306E5C303030645C3030306F5C3030306D5C3030302D5C303030415C303030675C303030655C3030306E5C303030745C3030305C3034305C303030425C303030615C303030735C303030655C3030306C5C303030695C3030306E5C30303065}
\BKM@entry{id=18,dest={617070656E6469782E313334},srcline={601}}{5C3337365C3337375C303030415C303030645C303030645C303030695C303030745C303030695C3030306F5C3030306E5C303030615C3030306C5C3030305C3034305C303030525C303030655C303030735C303030755C3030306C5C303030745C30303073}
\@writefile{toc}{\contentsline {subsubsection}{\numberline {E.2.1}Autumn-Simulator Agent}{12}{subsubsection.131}\protected@file@percent }
\newlabel{sec:autumn-simulator-agent}{{E.2.1}{12}{Final Normalized Perplexity}{subsubsection.131}{}}
\newlabel{sec:autumn-simulator-agent@cref}{{[subsubsection][1][5,2]E.2.1}{[1][11][]12}{}{}{}}
\@writefile{toc}{\contentsline {paragraph}{Task-specific solvers.}{12}{subsubsection.131}\protected@file@percent }
\@writefile{toc}{\contentsline {subsubsection}{\numberline {E.2.2}Random-Agent Baseline}{12}{subsubsection.132}\protected@file@percent }
\newlabel{sec:random-agent-results}{{E.2.2}{12}{Final Normalized Perplexity}{subsubsection.132}{}}
\newlabel{sec:random-agent-results@cref}{{[subsubsection][2][5,2]E.2.2}{[1][12][]12}{}{}{}}
\csxdef {autonum@tab:random_agent_probabilitiesReferenced}{}
\@writefile{lot}{\contentsline {table}{\numberline {E.1}{\ignorespaces Random-agent baseline by environment. Environments 1--26 are deterministic; 27--43 are stochastic. Columns report the probability of triggering the change within 1000 timesteps (CD) and reaching the goal within 1000 timesteps (PL).}}{12}{table.caption.133}\protected@file@percent }
\newlabel{tab:random_agent_probabilities}{{E.1}{12}{Random-agent baseline by environment. Environments 1--26 are deterministic; 27--43 are stochastic. Columns report the probability of triggering the change within 1000 timesteps (CD) and reaching the goal within 1000 timesteps (PL)}{table.caption.133}{}}
\newlabel{tab:random_agent_probabilities@cref}{{[table][1][5]E.1}{[1][12][]12}{}{}{}}
\BKM@entry{id=19,dest={73756273656374696F6E2E313335},srcline={609}}{5C3337365C3337375C303030445C303030655C303030745C303030615C303030695C3030306C5C303030655C303030645C3030305C3034305C303030505C303030655C303030725C303030665C3030306F5C303030725C3030306D5C303030615C3030306E5C303030635C303030655C3030305C3034305C303030415C3030306E5C303030615C3030306C5C303030795C303030735C303030695C30303073}
\BKM@entry{id=20,dest={73756273756273656374696F6E2E313336},srcline={614}}{5C3337365C3337375C303030505C303030655C303030725C3030302D5C303030455C3030306E5C303030765C303030695C303030725C3030306F5C3030306E5C3030306D5C303030655C3030306E5C303030745C3030305C3034305C303030535C303030635C3030306F5C303030725C303030655C30303073}
\BKM@entry{id=21,dest={73756273756273656374696F6E2E313337},srcline={625}}{5C3337365C3337375C303030505C303030725C3030306F5C3030306D5C303030705C303030745C3030305C3034305C303030525C3030306F5C303030625C303030755C303030735C303030745C3030306E5C303030655C303030735C303030735C3030305C3034305C303030415C3030306E5C303030615C3030306C5C303030795C303030735C303030695C30303073}
\citation{autumnbench_dataset}
\BKM@entry{id=22,dest={73756273756273656374696F6E2E313430},srcline={652}}{5C3337365C3337375C303030505C303030655C303030725C303030665C3030306F5C303030725C3030306D5C303030615C3030306E5C303030635C303030655C3030305C3034305C303030765C303030655C303030725C303030735C303030755C303030735C3030305C3034305C303030435C3030306F5C3030306D5C303030705C303030755C303030745C303030615C303030745C303030695C3030306F5C3030306E5C303030615C3030306C5C3030305C3034305C303030435C3030306F5C303030735C30303074}
\@writefile{toc}{\contentsline {section}{\numberline {F}Additional Results}{13}{appendix.134}\protected@file@percent }
\newlabel{sec:additional_results}{{F}{13}{Final Normalized Perplexity}{appendix.134}{}}
\newlabel{sec:additional_results@cref}{{[appendix][6][]F}{[1][12][]13}{}{}{}}
\csxdef {autonum@sec:detailed-performanceReferenced}{}
\csxdef {autonum@sec:behavioral-analysisReferenced}{}
\csxdef {autonum@sec:context-usageReferenced}{}
\csxdef {autonum@sec:external-correlationsReferenced}{}
\csxdef {autonum@sec:qualitative-examplesReferenced}{}
\@writefile{toc}{\contentsline {subsection}{\numberline {F.1}Detailed Performance Analysis}{13}{subsection.135}\protected@file@percent }
\newlabel{sec:detailed-performance}{{F.1}{13}{Final Normalized Perplexity}{subsection.135}{}}
\newlabel{sec:detailed-performance@cref}{{[appendix][1][6]F.1}{[1][13][]13}{}{}{}}
\csxdef {autonum@sec:per-env-scoresReferenced}{}
\csxdef {autonum@sec:cost-performanceReferenced}{}
\csxdef {autonum@sec:prompt-robustnessReferenced}{}
\@writefile{toc}{\contentsline {subsubsection}{\numberline {F.1.1}Per-Environment Scores}{13}{subsubsection.136}\protected@file@percent }
\newlabel{sec:per-env-scores}{{F.1.1}{13}{Final Normalized Perplexity}{subsubsection.136}{}}
\newlabel{sec:per-env-scores@cref}{{[subsubsection][1][6,1]F.1.1}{[1][13][]13}{}{}{}}
\csxdef {autonum@tab:avg_scoresReferenced}{}
\@writefile{toc}{\contentsline {paragraph}{Saturation check with Claude~Opus~4.6.}{13}{subsubsection.136}\protected@file@percent }
\csxdef {autonum@tab:avg_scoresReferenced}{}
\@writefile{toc}{\contentsline {subsubsection}{\numberline {F.1.2}Prompt Robustness Analysis}{13}{subsubsection.137}\protected@file@percent }
\newlabel{sec:prompt-robustness}{{F.1.2}{13}{Final Normalized Perplexity}{subsubsection.137}{}}
\newlabel{sec:prompt-robustness@cref}{{[subsubsection][2][6,1]F.1.2}{[1][13][]13}{}{}{}}
\@writefile{lot}{\contentsline {table}{\numberline {F.1}{\ignorespaces Performance of reasoning models under different prompts on a subset of AutumnBench problems}}{13}{table.caption.138}\protected@file@percent }
\newlabel{tab:prompt_comparison_subset}{{F.1}{13}{Performance of reasoning models under different prompts on a subset of AutumnBench problems}{table.caption.138}{}}
\newlabel{tab:prompt_comparison_subset@cref}{{[table][1][6]F.1}{[1][13][]13}{}{}{}}
\csxdef {autonum@tab:prompt_comparison_subsetReferenced}{}
\BKM@entry{id=23,dest={73756273656374696F6E2E313432},srcline={731}}{5C3337365C3337375C303030425C303030655C303030685C303030615C303030765C303030695C3030306F5C303030725C303030615C3030306C5C3030305C3034305C303030415C3030306E5C303030615C3030306C5C303030795C303030735C303030695C30303073}
\@writefile{toc}{\contentsline {subsubsection}{\numberline {F.1.3}Performance versus Computational Cost}{14}{subsubsection.140}\protected@file@percent }
\newlabel{sec:cost-performance}{{F.1.3}{14}{Final Normalized Perplexity}{subsubsection.140}{}}
\newlabel{sec:cost-performance@cref}{{[subsubsection][3][6,1]F.1.3}{[1][13][]14}{}{}{}}
\@writefile{toc}{\contentsline {paragraph}{Overall findings.}{14}{subsubsection.140}\protected@file@percent }
\@writefile{toc}{\contentsline {paragraph}{Task-specific patterns.}{14}{subsubsection.140}\protected@file@percent }
\@writefile{toc}{\contentsline {paragraph}{Environment characteristics.}{14}{subsubsection.140}\protected@file@percent }
\csxdef {autonum@tab:random_agent_probabilitiesReferenced}{}
\@writefile{lot}{\contentsline {table}{\numberline {F.2}{\ignorespaces Average scores by environment across three task types and agents. Qwen refers to Qwen3-235B-A22B-Thinking-2507.}}{14}{table.caption.141}\protected@file@percent }
\newlabel{tab:avg_scores}{{F.2}{14}{Average scores by environment across three task types and agents. Qwen refers to Qwen3-235B-A22B-Thinking-2507}{table.caption.141}{}}
\newlabel{tab:avg_scores@cref}{{[table][2][6]F.2}{[1][14][]14}{}{}{}}
\BKM@entry{id=24,dest={73756273756273656374696F6E2E313433},srcline={736}}{5C3337365C3337375C303030415C303030635C303030745C303030695C3030306F5C3030306E5C3030302D5C303030445C303030695C303030735C303030745C303030725C303030695C303030625C303030755C303030745C303030695C3030306F5C3030306E5C3030305C3034305C303030415C3030306E5C303030615C3030306C5C303030795C303030735C303030695C30303073}
\BKM@entry{id=25,dest={73756273756273656374696F6E2E313435},srcline={805}}{5C3337365C3337375C3030304F5C3030306E5C3030302D5C303030435C3030306C5C303030615C303030755C303030735C303030655C3030305C3034305C303030435C3030306F5C303030765C303030655C303030725C303030615C303030675C30303065}
\@writefile{toc}{\contentsline {subsection}{\numberline {F.2}Behavioral Analysis}{15}{subsection.142}\protected@file@percent }
\newlabel{sec:behavioral-analysis}{{F.2}{15}{Final Normalized Perplexity}{subsection.142}{}}
\newlabel{sec:behavioral-analysis@cref}{{[appendix][2][6]F.2}{[1][14][]15}{}{}{}}
\csxdef {autonum@sec:resultsReferenced}{}
\@writefile{toc}{\contentsline {subsubsection}{\numberline {F.2.1}Action-Distribution Analysis}{15}{subsubsection.143}\protected@file@percent }
\newlabel{sec:action-distribution}{{F.2.1}{15}{Final Normalized Perplexity}{subsubsection.143}{}}
\newlabel{sec:action-distribution@cref}{{[subsubsection][1][6,2]F.2.1}{[1][15][]15}{}{}{}}
\@writefile{lot}{\contentsline {table}{\numberline {F.3}{\ignorespaces Unique clicks and directional actions by environment and agent. Qwen refers to Qwen3-235B-A22B-Thinking-2507.}}{15}{table.caption.144}\protected@file@percent }
\newlabel{tab:avg_actions}{{F.3}{15}{Unique clicks and directional actions by environment and agent. Qwen refers to Qwen3-235B-A22B-Thinking-2507}{table.caption.144}{}}
\newlabel{tab:avg_actions@cref}{{[table][3][6]F.3}{[1][15][]15}{}{}{}}
\csxdef {autonum@tab:avg_actionsReferenced}{}
\@writefile{toc}{\contentsline {subsubsection}{\numberline {F.2.2}On-Clause Coverage}{15}{subsubsection.145}\protected@file@percent }
\newlabel{sec:coverage}{{F.2.2}{15}{Final Normalized Perplexity}{subsubsection.145}{}}
\newlabel{sec:coverage@cref}{{[subsubsection][2][6,2]F.2.2}{[1][15][]15}{}{}{}}
\BKM@entry{id=26,dest={73756273756273656374696F6E2E313436},srcline={812}}{5C3337365C3337375C303030525C303030655C303030735C303030655C303030745C3030305C3034305C303030535C303030655C303030715C303030755C303030655C3030306E5C303030635C303030655C3030305C3034305C303030415C3030306E5C303030615C3030306C5C303030795C303030735C303030695C30303073}
\citation{coenen2015strategies,bramley2018intuitive}
\BKM@entry{id=27,dest={73756273756273656374696F6E2E313438},srcline={842}}{5C3337365C3337375C303030435C3030306F5C3030306E5C303030745C303030655C303030785C303030745C3030302D5C3030304C5C303030655C3030306E5C303030675C303030745C303030685C3030305C3034305C303030535C303030635C303030615C3030306C5C303030695C3030306E5C30303067}
\citation{wang2026context}
\BKM@entry{id=28,dest={73756273656374696F6E2E313439},srcline={847}}{5C3337365C3337375C303030435C3030306F5C3030306E5C303030745C303030655C303030785C303030745C3030305C3034305C303030555C303030735C303030615C303030675C303030655C3030305C3034305C303030415C3030306E5C303030615C3030306C5C303030795C303030735C303030695C30303073}
\@writefile{toc}{\contentsline {subsubsection}{\numberline {F.2.3}Reset Sequence Analysis}{16}{subsubsection.146}\protected@file@percent }
\newlabel{sec:lcs-analysis}{{F.2.3}{16}{Final Normalized Perplexity}{subsubsection.146}{}}
\newlabel{sec:lcs-analysis@cref}{{[subsubsection][3][6,2]F.2.3}{[1][16][]16}{}{}{}}
\@writefile{lot}{\contentsline {table}{\numberline {F.4}{\ignorespaces LCS ratio between pre- and post-reset action sequences with adaptive windows sized to $6\%$ of interaction length, clipped to $[10, 50]$ actions. Higher values indicate more structured resets. All human--model differences significant at $p<10^{-18}$ under the Mann--Whitney U test.}}{16}{table.caption.147}\protected@file@percent }
\newlabel{tab:lcs_ratio}{{F.4}{16}{LCS ratio between pre- and post-reset action sequences with adaptive windows sized to $6\%$ of interaction length, clipped to $[10, 50]$ actions. Higher values indicate more structured resets. All human--model differences significant at $p<10^{-18}$ under the Mann--Whitney U test}{table.caption.147}{}}
\newlabel{tab:lcs_ratio@cref}{{[table][4][6]F.4}{[1][16][]16}{}{}{}}
\csxdef {autonum@tab:lcs_ratioReferenced}{}
\@writefile{toc}{\contentsline {subsubsection}{\numberline {F.2.4}Context-Length Scaling}{16}{subsubsection.148}\protected@file@percent }
\newlabel{sec:context-scaling}{{F.2.4}{16}{Final Normalized Perplexity}{subsubsection.148}{}}
\newlabel{sec:context-scaling@cref}{{[subsubsection][4][6,2]F.2.4}{[1][16][]16}{}{}{}}
\@writefile{toc}{\contentsline {subsection}{\numberline {F.3}Context Usage Analysis}{16}{subsection.149}\protected@file@percent }
\newlabel{sec:context-usage}{{F.3}{16}{Final Normalized Perplexity}{subsection.149}{}}
\newlabel{sec:context-usage@cref}{{[appendix][3][6]F.3}{[1][16][]16}{}{}{}}
\csxdef {autonum@tab:context_usageReferenced}{}
\@writefile{lot}{\contentsline {table}{\numberline {F.5}{\ignorespaces Context usage per model. We measure tokens at the final test-phase turn, which includes the complete interaction history.}}{16}{table.caption.150}\protected@file@percent }
\newlabel{tab:context_usage}{{F.5}{16}{Context usage per model. We measure tokens at the final test-phase turn, which includes the complete interaction history}{table.caption.150}{}}
\newlabel{tab:context_usage@cref}{{[table][5][6]F.5}{[1][16][]16}{}{}{}}
\BKM@entry{id=29,dest={73756273656374696F6E2E313531},srcline={876}}{5C3337365C3337375C303030435C3030306F5C303030725C303030725C303030655C3030306C5C303030615C303030745C303030695C3030306F5C3030306E5C3030305C3034305C303030775C303030695C303030745C303030685C3030305C3034305C303030455C303030785C303030745C303030655C303030725C3030306E5C303030615C3030306C5C3030305C3034305C303030425C303030655C3030306E5C303030635C303030685C3030306D5C303030615C303030725C3030306B5C30303073}
\citation{li24simpler}
\citation{jimenez2024swebench}
\citation{terminalbench}
\citation{rein2024gpqa}
\BKM@entry{id=30,dest={73756273656374696F6E2E313533},srcline={911}}{5C3337365C3337375C303030515C303030755C303030615C3030306C5C303030695C303030745C303030615C303030745C303030695C303030765C303030655C3030305C3034305C303030455C303030785C303030615C3030306D5C303030705C3030306C5C303030655C30303073}
\@writefile{toc}{\contentsline {subsection}{\numberline {F.4}Correlation with External Benchmarks}{17}{subsection.151}\protected@file@percent }
\newlabel{sec:external-correlations}{{F.4}{17}{Final Normalized Perplexity}{subsection.151}{}}
\newlabel{sec:external-correlations@cref}{{[appendix][4][6]F.4}{[1][17][]17}{}{}{}}
\csxdef {autonum@tab:external_correlationsReferenced}{}
\@writefile{lot}{\contentsline {table}{\numberline {F.6}{\ignorespaces AutumnBench scores alongside external benchmark scores, with Spearman $\rho $ correlations. \textsuperscript  {*}$p < 0.05$, \textsuperscript  {**}$p < 0.001$.}}{17}{table.caption.152}\protected@file@percent }
\newlabel{tab:external_correlations}{{F.6}{17}{AutumnBench scores alongside external benchmark scores, with Spearman $\rho $ correlations. \textsuperscript {*}$p < 0.05$, \textsuperscript {**}$p < 0.001$}{table.caption.152}{}}
\newlabel{tab:external_correlations@cref}{{[table][6][6]F.6}{[1][17][]17}{}{}{}}
\@writefile{toc}{\contentsline {subsection}{\numberline {F.5}Qualitative Examples}{17}{subsection.153}\protected@file@percent }
\newlabel{sec:qualitative-examples}{{F.5}{17}{Final Normalized Perplexity}{subsection.153}{}}
\newlabel{sec:qualitative-examples@cref}{{[appendix][5][6]F.5}{[1][17][]17}{}{}{}}
\csxdef {autonum@lst:mfp-promptReferenced}{}
\csxdef {autonum@lst:change-detection-promptReferenced}{}
\csxdef {autonum@lst:planning-promptReferenced}{}
\csxdef {autonum@lst:example_scratchpadReferenced}{}
\csxdef {autonum@lst:mfp_choicesReferenced}{}
\@writefile{lol}{\contentsline {lstlisting}{tables/scratchpad\textunderscore \textunderscore claude\textunderscore mfp\textunderscore exp\textunderscore particles.txt}{18}{lstlisting.154}\protected@file@percent }
\bibstyle{icml2026}
\bibdata{main}
\bibcite{autumnbench_dataset}{{1}{2025}{{Anonymous}}{{}}}
\bibcite{bramley2018intuitive}{{2}{2018}{{Bramley et~al.}}{{Bramley, Gerstenberg, Tenenbaum, and Gureckis}}}
\bibcite{coenen2015strategies}{{3}{2015}{{Coenen et~al.}}{{Coenen, Rehder, and Gureckis}}}
\bibcite{autumnsynth}{{4}{2023}{{Das et~al.}}{{Das, Tenenbaum, Solar-Lezama, and Tavares}}}
\bibcite{dreamerv3}{{5}{2025}{{Hafner et~al.}}{{Hafner, Pasukonis, Ba, and Lillicrap}}}
\bibcite{jimenez2024swebench}{{6}{2024}{{Jimenez et~al.}}{{Jimenez, Yang, Wettig, Yao, Pei, Press, and Narasimhan}}}
\bibcite{li24simpler}{{7}{2024}{{Li et~al.}}{{Li, Hsu, Gu, Pertsch, Mees, Walke, Fu, Lunawat, Sieh, Kirmani, Levine, Wu, Finn, Su, Vuong, and Xiao}}}
\bibcite{terminalbench}{{8}{2026}{{Merrill et~al.}}{{Merrill, Shaw, Carlini, Li, Raj, Bercovich, Shi, Shin, Walshe, Buchanan, Shen, Ye, Lin, Poulos, Wang, Jitsev, Nezhurina, Lu, Mastromichalakis, Xu, Chen, Liu, Zhang, Chen, Kashyap, Uslu, Li, Wu, Yan, Bian, Sharma, Sun, Dillmann, Anand, Lanpouthakoun, Koopah, Hu, Guha, Dreiman, Zhu, Krauth, Zhong, Muennighoff, Amanfu, Tan, Pimpalgaonkar, Aggarwal, Lin, Lan, Zhao, Liang, Wang, Wang, Zhou, Heineman, Liu, Trivedi, Yang, Lin, Shetty, Yang, Omi, Raoof, Li, Zhuo, Lin, Dai, Wang, Chai, Zhou, Wahdany, She, Hu, Dong, Zhu, Cui, Saiyed, Kolbeinsson, Rytting, Marten, Wang, Dimakis, Konwinski, and Schmidt}}}
\bibcite{rein2024gpqa}{{9}{2024}{{Rein et~al.}}{{Rein, Hou, Stickland, Petty, Pang, Dirani, Michael, and Bowman}}}
\bibcite{wang2026context}{{10}{2026}{{Wang et~al.}}{{Wang, Chen, Zhong, Zheng, Shao, Yu, Liu, Wang, Ding, Cao, and Kang}}}
\@writefile{lol}{\contentsline {listing}{\numberline {F.1}{\ignorespaces Example scratchpad for the \obfsname  {exp\_particles} environment, with choices listed in \autonum@processReference {autonum@referenceCrefOld}{forcsvlist}{lst:mfp_choices}.}}{21}{listing.405}\protected@file@percent }
\csxdef {autonum@lst:mfp_choicesReferenced}{}
\newlabel{lst:example_scratchpad}{{F.1}{21}{Example scratchpad for the \obfsname {exp\_particles} environment, with choices listed in \Cref {lst:mfp_choices}}{listing.405}{}}
\newlabel{lst:example_scratchpad@cref}{{[listing][1][6]F.1}{[1][21][]21}{}{}{}}
\@writefile{lol}{\contentsline {listing}{\numberline {F.2}{\ignorespaces Answer choices, indexed 0--5, supplied for masked frame prediction in the \obfsname  {exp\_particles} environment.}}{22}{listing.caption.406}\protected@file@percent }
\newlabel{lst:mfp_choices}{{F.2}{22}{Answer choices, indexed 0--5, supplied for masked frame prediction in the \obfsname {exp\_particles} environment}{listing.caption.406}{}}
\newlabel{lst:mfp_choices@cref}{{[listing][2][6]F.2}{[1][21][]22}{}{}{}}
\gdef \@abspage@last{22}
\end{filecontents}
